# Supplementary material for: DEWP: Deep Expansion Learning for Wind Power Forecasting
Source: arXiv:2401.00644 source file (2024-01-01)
Supplement: Supplementary file 1 [file 7_appendix.tex]

\appendix

\section{Appendix Experiments}

To further verify and demonstrate the scalability of the proposed DEWP framework, we conduct the experiments on another wind power dataset of three-year length. Specifically, this dataset is named GER, which is collected at a wind farm in German ranging from 2017 to 2019. We collect the raw wind power data from the OPSD\footnote{{https://open-power-system-data.org}} and process the raw data similar to the above two benchmarks. GER dataset is of three-year length which is longer than the original two benchmarks. GER dataset includes wind capacity (Electrical Capacity of wind Turbine) as extra feature input, in addition to the temperatures, etc. 

We conduct the extra experiments on the above GER dataset on short-term and long-term forecasting tasks. More experimental results are in Table \ref{tab:append1} and Table \ref{tab:append2}. Experimental results show that our DEWP still outperforms other baseline algorithms in GER dataset, which signifies our consistent superiority in wind power forecasting. Moreover, we notice that with the increase of lookback size, the forecasting performance becomes worse. This shows the noisy wind power data would bring much errors that influence forecasting.

\begin{table*}[t]
\small
\centering
\caption{Overall performance comparisons of \textsc{Short-Term} wind power forecasting on GER dataset.}
\begin{tabular}{c|ccc|ccc}
%\hline \textbf{Datasets} & \multicolumn{6}{|c}{ \textbf{R80736} } \\
\hline \textbf{Lookback} & \multicolumn{3}{|c|}{ \textbf{24} } & \multicolumn{3}{c}{ \textbf{72} } \\
\hline \diagbox{\textbf{Method}}{\textbf{Metrics}} & \textbf{MAPE} & \textbf{MSPE} & \textbf{MAE} & \textbf{MAPE} & \textbf{MSPE} & \textbf{MAE}  \\
\hline
WPF-GRN & 6.112 & 30.33 & 0.5328 & 7.322 & 51.34 & 0.6291 \\
WPF-TSA & 5.787 & 27.23 & 0.5231 & 6.217 & 52.16 & 0.6131 \\
Informer &5.713 & 28.77 & 0.5133 & 6.110 & 48.65 &0.5490  \\
N-BEATS & 5.633 & 29.52 & 0.5003 & 5.993 & 47.31 &0.5520      \\
\hline 
\textbf{DEWP}   & \textbf{5.238} & \textbf{26.82} & \textbf{0.4930} & \textbf{5.373} & \textbf{44.23} & \textbf{0.5203} \\
\hline
\end{tabular}
\label{tab:append1}
\end{table*}

\begin{table*}[t]
\small
\centering
\caption{Overall performance comparisons of \textsc{Long-Term} wind power forecasting on GER dataset.}
\begin{tabular}{c|ccc|ccc}
%\hline \textbf{Datasets} & \multicolumn{6}{|c}{ \textbf{R80736} } \\
\hline \textbf{Lookback} & \multicolumn{3}{|c|}{ \textbf{48} } & \multicolumn{3}{c}{ \textbf{72} } \\
\hline \diagbox{\textbf{Method}}{\textbf{Metrics}} & \textbf{MAPE} & \textbf{MSPE} & \textbf{MAE} & \textbf{MAPE} & \textbf{MSPE} & \textbf{MAE}  \\
\hline
WPF-GRN & 7.112 & 41.24 & 0.7828 & 8.232 & 56.59 & 0.8294 \\
WPF-TSA & 6.347 & 37.23 & 0.7713 & 8.183 & 58.63 & 0.8101 \\
Informer &6.133 & 38.47 & 0.7821 & 7.101 & 58.71 &0.8393  \\
N-BEATS & 6.013 & 37.12 & 0.7424 & 6.993 & 56.29 &0.8027      \\
\hline 
\textbf{DEWP}   & \textbf{5.934} & \textbf{35.75} & \textbf{0.7383} & \textbf{6.387} & \textbf{49.09} & \textbf{0.7914}\\
\hline
\end{tabular}
\label{tab:append2}
\end{table*}
